# Supplementary material for: Relational Proxies: Emergent Relationships as Fine-Grained Discriminators
Source: arXiv:2210.02149 source file (2022-10-05)
Supplement: Supplementary file 1 [file bibliography_supp.tex]

@String(PAMI = {IEEE Trans. Pattern Anal. Mach. Intell.})
@String(IJCV = {Int. J. Comput. Vis.})
@String(CVPR= {IEEE Conf. Comput. Vis. Pattern Recog.})
@String(ICCV= {Int. Conf. Comput. Vis.})
@String(ECCV= {Eur. Conf. Comput. Vis.})
@String(NIPS= {Adv. Neural Inform. Process. Syst.})
@String(ICPR = {Int. Conf. Pattern Recog.})
@String(BMVC= {Brit. Mach. Vis. Conf.})
@String(TOG= {ACM Trans. Graph.})
@String(TIP  = {IEEE Trans. Image Process.})
@String(TVCG  = {IEEE Trans. Vis. Comput. Graph.})
@String(TMM  = {IEEE Trans. Multimedia})
@String(ACMMM= {ACM Int. Conf. Multimedia})
@String(ICME = {Int. Conf. Multimedia and Expo})
@String(ICASSP=	{ICASSP})
@String(ICIP = {IEEE Int. Conf. Image Process.})
@String(ACCV  = {ACCV})
@String(ICLR = {Int. Conf. Learn. Represent.})
@String(IJCAI = {IJCAI})
@String(PR   = {Pattern Recognition})
@String(AAAI = {AAAI})
@String(CVPRW= {IEEE Conf. Comput. Vis. Pattern Recog. Worksh.})
@String(CSVT = {IEEE Trans. Circuit Syst. Video Technol.})

@String(SPL	= {IEEE Sign. Process. Letters})
@String(VR   = {Vis. Res.})
@String(JOV	 = {J. Vis.})
@String(TVC  = {The Vis. Comput.})
@String(JCST  = {J. Comput. Sci. Tech.})
@String(CGF  = {Comput. Graph. Forum})
@String(CVM = {Computational Visual Media})


@String(PAMI  = {IEEE TPAMI})
@String(IJCV  = {IJCV})
@String(CVPR  = {CVPR})
@String(ICCV  = {ICCV})
@String(ECCV  = {ECCV})
@String(NIPS  = {NeurIPS})
@String(ICPR  = {ICPR})
@String(BMVC  =	{BMVC})
@String(TOG   = {ACM TOG})
@String(TIP   = {IEEE TIP})
@String(TVCG  = {IEEE TVCG})
@String(TCSVT = {IEEE TCSVT})
@String(TMM   =	{IEEE TMM})
@String(ACMMM = {ACM MM})
@String(ICME  =	{ICME})
@String(ICASSP=	{ICASSP})
@String(ICIP  = {ICIP})
@String(ACCV  = {ACCV})
@String(ICLR  = {ICLR})
@String(IJCAI = {IJCAI})
@String(PR = {PR})
@String(AAAI = {AAAI})
@String(CVPRW= {CVPRW})
@String(CSVT = {IEEE TCSVT})

@InProceedings{Angelova2013DetectSegment,
author={Angelova, Anelia and Zhu, Shenghuo},
booktitle={CVPR},
title={Efficient Object Detection and Segmentation for Fine-Grained Recognition},
year={2013}}

@InProceedings{Zhang2014RcnnFgvc,
author={Zhang, Ning and Donahue, Jeff and Girshick, Ross and Darrell, Trevor},
title="Part-Based R-CNNs for Fine-Grained Category Detection",
booktitle="ECCV",
year="2014",
}

@InProceedings{Lin2015DeepLAC,
author={Lin, Di and Shen, Xiaoyong and Lu, Cewu and Jia, Jiaya},
booktitle={CVPR},
title={Deep LAC: Deep localization, alignment and classification for fine-grained recognition},   year={2015}
}

@inproceedings{Branson2014PoseNorm,
   author = {Steve Branson and Grant Van Horn and Serge Belongie and Pietro Perona},
   booktitle = {BMVC},
   title = {Bird species categorization using pose normalized deep convolutional nets},
   year = {2014},
}

@inproceedings{Cui2016FgvcDml,
   author = {Yin Cui and Feng Zhou and Yuanqing Lin and Serge Belongie},
   booktitle = {CVPR},
   title = {Fine-grained categorization and dataset bootstrapping using deep metric learning with humans in the loop},
   year = {2016},
}

@inproceedings{Moghimi2016BoostedCNN,
   author = {Mohammad Moghimi and Mohammad Saberian and Jian Yang and Li Jia Li and Nuno Vasconcelos and Serge Belongie},
   booktitle = {BMVC},
   title = {Boosted convolutional neural networks},
   year = {2016},
}

@inproceedings{Cui2017,
   author = {Yin Cui and Feng Zhou and Jiang Wang and Xiao Liu and Yuanqing Lin and Serge Belongie},
   booktitle = {CVPR},
   title = {Kernel pooling for convolutional neural networks},
   year = {2017},
}

@inproceedings{Luo2019CrossX,
   author = {Wei Luo and Xitong Yang and Xianjie Mo and Yuheng Lu and Larry Davis and Jun Li and Jian Yang and Ser Nam Lim},
   booktitle = {ICCV},
   title = {Cross-X learning for fine-grained visual categorization},
   year = {2019},
}

@inproceedings{Zhang2021MMAL,
   author = {Fan Zhang and Meng Li and Guisheng Zhai and Yizhao Liu},
   booktitle = {MMM},
   title = {{Multi-branch and Multi-scale Attention Learning for Fine-Grained Visual Categorization}},
   year = {2021},
}

@inproceedings{Behera2021CAP,
   author = {Ardhendu Behera and Zachary Wharton and Asish Bera},
   booktitle = {AAAI},
   title = {{Context-aware Attentional Pooling (CAP) for Fine-grained Visual Classification}},
   year = {2021},
}

@inproceedings{Ding2021CDB,
   author = {Yifeng Ding and Shuwei Dong and Yujun Tong and Zhanyu Ma and Bo Xiao and Haibin Ling},
   booktitle = {BMVC},
   title = {{Channel DropBlock: An Improved Regularization Method for Fine-Grained Visual Classification}},
   year = {2021},
}

@inproceedings{Wang2021FFVT,
   author = {Jun Wang and Xiaohan Yu and Yongsheng Gao},
   booktitle = {BMVC},
   title = {{Feature Fusion Vision Transformer for Fine-Grained Visual Categorization}},
   year = {2021},
}

@inproceedings{He2022TransFG,
   author = {Ju He and Jie-Neng Chen and Shuai Liu and Adam Kortylewski and Cheng Yang and Yutong Bai and Changhu Wang},
   booktitle = {AAAI},
   title = {{TransFG: A Transformer Architecture for Fine-grained Recognition}},
   year = {2022},
}

@inproceedings{Lu2021SwinFGHash,
   author = {Di Lu and Jinpeng Wang and Ziyun Zeng and Bin Chen and Shudeng Wu and Shu-Tao Xia},
   booktitle = {BMVC},
   title = {{SwinFGHash: Fine-grained Image Retrieval via Transformer-based Hashing Network}},
   year = {2021},
}

@inproceedings{Vaswani2017,
   author = {Ashish Vaswani and Noam Shazeer and Niki Parmar and Jakob Uszkoreit and Llion Jones and Aidan N. Gomez and Łukasz Kaiser and Illia Polosukhin},
   booktitle = {NeurIPS},
   title = {An image is worth 16x16 words: transformers for image recognition at scale},
   year = {2017},
}

@inproceedings{Zambaldi2019RelationRL,
   author = {Vinicius Zambaldi and David Raposo and Adam Santoro and Victor Bapst and Yujia Li and Igor Babuschkin and Karl Tuyls and David Reichert and Timothy Lillicrap and Edward Lockhart and Murray Shanahan and Victoria Langston and Razvan Pascanu and Matthew Botvinick and Oriol Vinyals and Peter Battaglia},
   booktitle = {ICLR},
   title = {Deep reinforcement learning with relational inductive biases},
   year = {2019},
}

@inproceedings{Hu2018RelationOD,
   author = {Han Hu and Jiayuan Gu and Zheng Zhang and Jifeng Dai and Yichen Wei},
   booktitle = {CVPR},
   title = {{Relation Networks for Object Detection}},
   year = {2018},
}

@inproceedings{Santoro2019RelationQA,
   author = {Adam Santoro and David Raposo and David G.T. Barrett and Mateusz Malinowski and Razvan Pascanu and Peter Battaglia and Timothy Lillicrap},
   booktitle = {NeurIPS},
   title = {A simple neural network module for relational reasoning},
   year = {2017},
}

@article{Battaglia2018RelationGraphs,
   author = {Peter W. Battaglia and Jessica B. Hamrick and Victor Bapst and Alvaro Sanchez-Gonzalez and Vinicius Zambaldi and Mateusz Malinowski and Andrea Tacchetti and David Raposo and Adam Santoro and Ryan Faulkner and Caglar Gulcehre and Francis Song and Andrew Ballard and Justin Gilmer and George Dahl and Ashish Vaswani and Kelsey Allen and Charles Nash and Victoria Langston and Chris Dyer and Nicolas Heess and Daan Wierstra and Pushmeet Kohli and Matt Botvinick and Oriol Vinyals and Yujia Li and Razvan Pascanu},
   month = {6},
   title = {Relational inductive biases, deep learning, and graph networks},
   url = {http://arxiv.org/abs/1806.01261},
   journal	= {arXiv},
   year = {2018},
}

@inproceedings{Sung2018RelationFSL,
   author = {Flood Sung and Yongxin Yang and Li Zhang and Tao Xiang and Philip H.S. Torr and Timothy M. Hospedales},
   booktitle = {CVPR},
   title = {{Learning to Compare: Relation Network for Few-Shot Learning}},
   year = {2018},
}

@inproceedings{Park2019RKD,
   author = {Wonpyo Park and Dongju Kim and Yan Lu and Minsu Cho},
   booktitle = {CVPR},
   title = {Relational knowledge distillation},
   year = {2019},
}

@inproceedings{Patacchiola2022RelationalReasoningSSL,
   author = {Massimiliano Patacchiola and Amos Storkey},
   booktitle = {NeurIPS},
   title = {Self-supervised relational reasoning for representation learning},
   year = {2020},
}

@inproceedings{Movshovitz-Attias2017ProxyNCA,
   author = {Yair Movshovitz-Attias and Alexander Toshev and Thomas K. Leung and Sergey Ioffe and Saurabh Singh},
   booktitle = {ICCV},
   title = {{No Fuss Distance Metric Learning Using Proxies}},
   year = {2017},
}

@inproceedings{Teh2020ProxyNCApp,
   author = {Eu Wern Teh and Terrance DeVries and Graham W. Taylor},
   booktitle = {ECCV},
   title = {{ProxyNCA++: Revisiting and Revitalizing Proxy Neighborhood Component Analysis}},
   year = {2020},
}

@inproceedings{Kim2020CVPR,
   author = {Sungyeon Kim and Dongwon Kim and Minsu Cho and Suha Kwak},
   booktitle = {CVPR},
   title = {Proxy anchor loss for deep metric learning},
   year = {2020},
}

@inproceedings{Roth2022NIR,
   author = {Karsten Roth and Oriol Vinyals and Zeynep Akata},
   booktitle = {CVPR},
   title = {{Non-isotropy Regularization for Proxy-based Deep Metric Learning}},
   year = {2022},
}

@inproceedings{Yang2022HierarchicalProxy,
   author = {Zhibo Yang and Muhammet Bastan and Xinliang Zhu and Doug Gray and Dimitris Samaras},
   booktitle = {WACV},
   title = {{Hierarchical Proxy-based Loss for Deep Metric Learning}},
   year = {2022},
}

@inproceedings{Choudhury2021UnsupervisedParts,
   author = {Subhabrata Choudhury and Iro Laina and Christian Rupprecht and Andrea Vedaldi},
   booktitle = {NeurIPS},
   title = {{Unsupervised Part Discovery from Contrastive Reconstruction}},
   year = {2021},
}

@inproceedings{Federici2020MIB,
   author = {Marco Federici and Anjan Dutta and Patrick Forré and Nate Kushman and Zeynep Akata},
   booktitle = {ICLR},
   title = {{Learning Robust Representations via Multi-View Information Bottleneck}},
   year = {2020},
}

@article{Wei2017SCDA,
   author = {Xiu Shen Wei and Jian Hao Luo and Jianxin Wu and Zhi Hua Zhou},
   journal = {IEEE TIP},
   title = {{Selective Convolutional Descriptor Aggregation for Fine-Grained Image Retrieval}},
   year = {2017},
}

@inproceedings{Naseer2021IntriguingViT,
   author = {Muzammal Naseer and Kanchana Ranasinghe and Salman Khan and Munawar Hayat and Fahad Shahbaz Khan and Ming-Hsuan Yang},
   booktitle = {NeurIPS},
   title = {{Intriguing Properties of Vision Transformers}},
   year = {2021},
}

@inproceedings{Caron2021DiNo,
   author = {Mathilde Caron and Hugo Touvron and Ishan Misra and Hervé Jégou and Julien Mairal and Piotr Bojanowski and Armand Joulin},
   booktitle = {NeurIPS},
   title = {{Emerging Properties in Self-Supervised Vision Transformers}},
   year = {2021},
}

@inproceedings{Huang2016PartStackedCNN,
   author = {Shaoli Huang and Zhe Xu and Dacheng Tao and Ya Zhang},
   booktitle = {CVPR},
   title = {Part-stacked CNN for fine-grained visual categorization},
   year = {2016},
}

@InProceedings{Paszke2017PyTorch,
    author    = {Paszke, Adam and Gross, Sam and Chintala, Soumith and Chanan, Gregory and Yang, Edward and DeVito, Zachary and Lin, Zeming and Desmaison, Alban and Antiga, Luca and Lerer, Adam},
    title     = {Automatic differentiation in {PyTorch}},
    booktitle = {NIPSW},
    year      = {2017},
}

@article{Maji2013FGVCAircraft,
  title={{Fine-Grained Visual Classification of Aircraft}},
  author={Subhransu Maji and Esa Rahtu and Juho Kannala and Matthew B. Blaschko and Andrea Vedaldi},
  journal={arXiv},
  year={2013}
}

@inproceedings{krause2013StanfordCars,
  title = {{3D Object Representations for Fine-Grained Categorization}},
  booktitle = {3DRR},
  year = {2013},
  author = {Jonathan Krause and Michael Stark and Jia Deng and Li Fei-Fei}
}

@inproceedings{Wah2011CUB,
  title={The Caltech-UCSD Birds-200-2011 Dataset},
  author={Catherine Wah and Steve Branson and Peter Welinder and Pietro Perona and Serge J. Belongie},
  booktitle = {California Institute of Technology, CNS-TR-2010-001},
  year={2011}
}

@inproceedings{horn2015NABirds,
  author={Van Horn, Grant and Branson, Steve and Farrell, Ryan and Haber, Scott and Barry, Jessie and Ipeirotis, Panos and Perona, Pietro and Belongie, Serge},
  booktitle={CVPR},
  title={Building a bird recognition app and large scale dataset with citizen scientists: The fine print in fine-grained dataset collection}, 
  year={2015},
}

@inproceedings{Yu2020SoyCottonCultivar,
  title={Patchy Image Structure Classification Using Multi-Orientation Region Transform},
  author={Xiaohan Yu and Yang Zhao and Yongsheng Gao and Shengwu Xiong and Xiaohui Yuan},
  booktitle={AAAI},
  year={2020}
}

@article{He2016DeepRL,
  title={Deep Residual Learning for Image Recognition},
  author={Kaiming He and X. Zhang and Shaoqing Ren and Jian Sun},
  journal={CVPR},
  year={2016}
}

@article{Deng2009ImageNetAL,
  title={ImageNet: A large-scale hierarchical image database},
  author={Jia Deng and Wei Dong and Richard Socher and Li-Jia Li and K. Li and Li Fei-Fei},
  journal={CVPR},
  year={2009},
}

@inproceedings{dubey2018MaxEntFGVC,
 author = {Dubey, Abhimanyu and Gupta, Otkrist and Raskar, Ramesh and Naik, Nikhil},
 booktitle = {NeurIPS},
 title = {Maximum-Entropy Fine Grained Classification},
 year = {2018}
}

@inproceedings{zheng2019DBT,
 author = {Zheng, Heliang and Fu, Jianlong and Zha, Zheng-Jun and Luo, Jiebo},
 booktitle = {NeurIPS},
 title = {Learning Deep Bilinear Transformation for Fine-grained Image Representation},
 year = {2019}
}

@inproceedings{kou2020StochNorm,
 author = {Kou, Zhi and You, Kaichao and Long, Mingsheng and Wang, Jianmin},
 booktitle = {NeurIPS},
 title = {Stochastic Normalization},
 year = {2020}
}

@inproceedings{zhang2016SPDACNN,
   author = {Han Zhang and Tao Xu and Mohamed Elhoseiny and Xiaolei Huang and Shaoting Zhang and Ahmed Elgammal and Dimitris Metaxas},
   booktitle = {CVPR},
   title = {SPDA-CNN: Unifying semantic part detection and abstraction for fine-grained recognition},
   year = {2016},
}

@article{wei2018MaskCNN,
   author = {Xiu Shen Wei and Chen Wei Xie and Jianxin Wu and Chunhua Shen},
   journal = {PR},
   title = {Mask-CNN: Localizing parts and selecting descriptors for fine-grained bird species categorization},
   year = {2018},
}

@inproceedings{lam2017HSNet,
   author = {Michael Lam and Behrooz Mahasseni and Sinisa Todorovic},
   booktitle = {CVPR},
   title = {Fine-grained recognition as hsnet search for informative image parts},
   year = {2017},
}

@InCollection{oconnor2021emergence,
	author       =	{O’Connor, Timothy},
	title        =	{{Emergent Properties}},
	booktitle    =	{The {Stanford} Encyclopedia of Philosophy},
	editor       =	{Edward N. Zalta},
	howpublished =	{\url{https://plato.stanford.edu/archives/win2021/entries/properties-emergent/}},
	year         =	{2021},
	edition      =	{{W}inter 2021},
	publisher    =	{Metaphysics Research Lab, Stanford University}
}

@inproceedings{Khosla2011StanfordDogs,
    author = "Aditya Khosla and Nityananda Jayadevaprakash and Bangpeng Yao and Li Fei-Fei",
    title = "Novel Dataset for Fine-Grained Image Categorization",
    booktitle = "CVPRW",
    year = "2011"
}

@misc{Li2017TinyImageNet,
    author = {Fei-Fei Li and Andrej Karpathy and Justin Johnson},
    title={Tiny Image Net},
    howpublished={\url{https://www.kaggle.com/c/tiny-imagenet}},
    year = {2017},
}

@article{mcinnes2018umap-software,
  title={{UMAP: Uniform Manifold Approximation and Projection}},
  author={McInnes, Leland and Healy, John and Saul, Nathaniel and Grossberger, Lukas},
  journal={JOSS},
  year={2018}
}

@InProceedings{Horn2018iNat,
    author = {Van Horn, Grant and Mac Aodha, Oisin and Song, Yang and Cui, Yin and Sun, Chen and Shepard, Alex and Adam, Hartwig and Perona, Pietro and Belongie, Serge},
    title = {{The iNaturalist Species Classification and Detection Dataset}},
    booktitle = {CVPR},
    year = {2018}
}

@InProceedings{Simonyan2015VGG16,
  author       = "Karen Simonyan and Andrew Zisserman",
  title        = "Very Deep Convolutional Networks for Large-Scale Image Recognition",
  booktitle    = "ICLR",
  year         = "2015",
}
